# Supplementary material for: HIT: A Hierarchically Fused Deep Attention Network for Robust Code-mixed Language Representation
Source: arXiv:2105.14600 source file (2021-05-30)
Supplement: Supplementary file 1 [file supplement.tex]

% %
% % File acl2021.tex
% %
% %% Based on the style files for EMNLP 2020, which were
% %% Based on the style files for ACL 2020, which were
% %% Based on the style files for ACL 2018, NAACL 2018/19, which were
% %% Based on the style files for ACL-2015, with some improvements
% %%  taken from the NAACL-2016 style
% %% Based on the style files for ACL-2014, which were, in turn,
% %% based on ACL-2013, ACL-2012, ACL-2011, ACL-2010, ACL-IJCNLP-2009,
% %% EACL-2009, IJCNLP-2008...
% %% Based on the style files for EACL 2006 by 
% %%e.agirre@ehu.es or Sergi.Balari@uab.es
% %% and that of ACL 08 by Joakim Nivre and Noah Smith

% \documentclass[11pt,a4paper]{article}
% \usepackage[hyperref]{acl2021}
% \usepackage{times}
% \usepackage{latexsym}
% \usepackage[linesnumbered,ruled]{algorithm2e}
% \usepackage{subfig}
% \usepackage{graphicx}
% \usepackage[T1]{fontenc}
% \usepackage{graphics}
% \usepackage{multirow}
% \usepackage{multicol}
% \usepackage{enumitem}
% \usepackage{soul,xcolor}
% \usepackage{amsmath}
% \usepackage{caption}
% \usepackage{subcaption}
% \usepackage{arydshln}
% \captionsetup{compatibility=false}
% %\usepackage{subfigure}
% %\usepackage{subfig}

% \renewcommand{\UrlFont}{\ttfamily\small}

% % This is not strictly necessary, and may be commented out,
% % but it will improve the layout of the manuscript,
% % and will typically save some space.
% \usepackage{microtype}

% \aclfinalcopy % Uncomment this line for the final submission
% %\def\aclpaperid{***} %  Enter the acl Paper ID here

% %\setlength\titlebox{5cm}
% % You can expand the titlebox if you need extra space
% % to show all the authors. Please do not make the titlebox
% % smaller than 5cm (the original size); we will check this
% % in the camera-ready version and ask you to change it back.
% \usepackage{tikz}
% \def\checkmark{\tikz\fill[scale=0.4](0,.35) -- (.25,0) -- (1,.7) -- (.25,.15) -- cycle;} 
% \usepackage{pifont}% http://ctan.org/pkg/pifont
% \newcommand{\cmark}{\ding{51}}%
% \newcommand{\xmark}{\ding{55}}%

% \newcommand\BibTeX{B\textsc{ib}\TeX}
% \newcommand{\name}{\textsf{HIT}}

% \title{\name: A Hierarchically Fused Deep Attention Network for Robust Code-mixed Language Representation \\ {(Appendix)}}

% \author{Ayan Sengupta$^1$, Sourabh Kumar Bhattacharjee$^1$, \\ \textbf{Tanmoy Chakraborty$^2$, Md Shad Akhtar$^2$} \\
%   $^1$Optum Global Advantage (UnitedHealth Group), Noida, India\\ 
% $^2$Dept. of CSE, IIIT-Delhi, India\\
%   \texttt{\{ayan.sengupta007, sourabhb398\}@gmail.com}; \\
%   \texttt{\{tanmoy, shad.akhtar\}@iiitd.ac.in} \\
%   }

% \date{}

% \begin{document}
% \maketitle

% \section{Semantic Understanding of Languages}\label{subs: semanticanalysis}

% In this section, we study the semantic relationships between different Indic languages. We calculate the proportion of common words in Table~\ref{tab:words} between different language pairs to understand the multilingualism in India. We observe that Bengali code-mixed texts have the highest proportion of English words $32\%$ as compared to other languages. Moreover, $50\%$ of all Bengali words are also present in the Hindi CM texts, although $58\%$ of those words are English. We observe that users using Hindi CM texts use very few words taken from other languages. On the other hand, a significant proportion of Bengali and Telugu CM words are common in other languages, although, majority of them are English. The two Dravidian languages, Tamil and Malayalam, show a very distinctive behavior. They share very little linguistic similarity with other Indic languages. On the other hand, $10\%$ of all Tamil words are used in Malayalam and $17\%$ of all Malayalam words are used in Tamil. Moreover, this sharing is not driven by English, as, only $27\%$ of these words are English, which is the lowest proportion among all other language pairs. Being originate from a similar root and having a phonetic resemblance makes Tamil and Malayalam \textit{sister languages}\footnote{\url{https://royalsocietypublishing.org/doi/10.1098/rsos.171504}}.
% \begin{figure}[ht!]
% %%\vspace*{-0.25cm}
%      \centering
%      \subfloat[]{\includegraphics[scale=.2]{images/tsne.pdf}}
     
%      %\hspace*{-1.5cm}
%      \subfloat[]{\includegraphics[scale=.2]{images/tsne_pronoun.pdf}}
%      \caption{t-SNE visualization (a) of all words;\, (b) of selected pronouns. Overlapping clusters show how semantically similar words from different languages are embedded onto a similar space.}
%      \label{fig:tsne}
% 		%\vspace*{-0.5cm}
% \end{figure}
% \input{tab-words}
% \begin{table*}[ht!]
%     \centering
%     \resizebox{\textwidth}{!}{
%     \begin{tabular}{c|p{40em}}
%          \textbf{Lang} & \textbf{POS tags} \\ \hline
%          Hindi (14) & \textit{X, VERB, NOUN, ADP, PROPN, ADJ, PART, PRON, DET, ADV, CONJ, PART\_NEG, PRON\_WH, NUM}\\ \hline
%          Bengali (39) & \textit{N\_NN, V\_VM, RD\_PUNC, N\_NNP, PSP, PR\_PRP, JJ, RB\_AMN, CC, QT\_QTF, DM\_DMD, RP\_RPD, @, RD\_RDF, V\_VAUX, DT, PR\_PRQ, \#, RP\_NEG, E, \$, RB\_ALC, N\_NNV, PR\_PRL, N\_NST, RP\_INJ, RD\_SYM, DM\_DMR, RP\_INTF, PR\_PRF, DM\_DMQ, QT\_QTO, U, QT\_QTC, PR\_PRC, RD\_ECH, QY\_QTO, Ã°Å¸Ëœ, $\sim$} \\ \hline
%          Telugu (52) & \textit{N\_NN, N\_NNP, RD\_RDF, RD\_PUNC, V\_VM, JJ, @, PSP, PR\_PRP, RP\_INJ, DT, RB\_AMN, CC, \$, U, E, \#, N\_NNV, \&, PR\_PRQ, V\_VAUX, RD\_PUNC", $\sim$, RD\_RDFP, QT\_QTF, RD\_UNK, DM\_DMD, RP\_RPD, RB\_ALC, DM\_DMQ, RD\_ECH, N\_NST, acro, PR\_PRL, QT\_QFC, RP\_RDF, PR\_PRC, r, RD\_SYM, RD\_RDFF, psp, PR\_PRF, QT\_QTP, RD\_P/UNC, PR\_PPR, PR\_RPQ, RPR\_PRP, RP\_INTF, -} \\ \hline
%          Spanish (17) & \textit{VERB, PUNCT, PRON, NOUN, DET, ADV, ADP, INTJ, CONJ, ADJ, AUX, SCONJ, PART, PROPN, NUM, UNK, X}\\ \hline
%     \end{tabular}}
%     \caption{POS tagsets for different datasets.}
%     \label{tab:tags}
% \end{table*}
% Similar observations are also made from the word representation lens. We use t-SNE~\cite{van2008visualizing} plots to embed {\name's} representations onto a $2$-D space for interpretability (Fig~\ref{fig:tsne}). Although, the embeddings are well clustered based on the languages, we can easily figure out the semantically similar words across languages embedded onto a similar space. Furthermore, Fig~\ref{fig:tsne}(b) shows that pronouns (e.g., \textit{`aap'}) in Tamil, Telegu and Hindi are embedded onto a similar space with Bengali words \textit{`aamar', `aamay'}. Although each of these representations are learned on separate models on separate datasets, the robustness of the underlying hierarchical representation enables our model to capture cross-lingual semantics from noisy code-mixed texts. We can attribute these observations to the relatedness of Indic languages on a socio-cultural basis.


% \section{Datasets}
% We report all available POS tags in Table \ref{tab:tags}.\\
% % $\bullet$  \textbf{Sentiment classification:} The Hindi-English and Spanish-English sentiment datasets contain 3 labels - \textit{positive}, \textit{negative} and \textit{neutral}. Both Tamil-English and Malayalam-English sentiment classification datasets contain \textit{Positive}, \textit{Negative}, \textit{Mixed\_feelings}, \textit{Unknown\_state}. Additionally, \textit{not-Tamil} and \textit{not-Malayalam} classes are present in the Ta-En and Ma-En dataset respectively. For Tamil-English and Malayalam-English sentiment analysis datasets we use the original test-dev-test split from ~\cite{chakravarthi-etal-2020-corpus, chakravarthi-etal-2020-sentiment}. For Spanish-English sentiment, we use dataset proposed by ~\cite{patwa-etal-2020-sentimix}. Although this dataset contains train-dev-test split, the ground truth labels are not provided for test datasets. Due to this reason, we use the dev dataset for testing for Sp-En sentiment classification task.\\
% % $\bullet$  \textbf{POS Tagging:}
% % Bengali code-mixed POS dataset contains total 39 fine-grained labels including. 
% % \\
% % Similarly, Telegu code-mixed POS dataset contains total 52 different classes which include .
% % \\
% % On the other hand, Hindi-English and Spanish-English NER datasets contain fewer labels, 14 and 18 respectively. 


% % \if 0
% % \section{Hyperparameters}
% % We report the optimal hyperparameters used in the experiments for different tasks in Table~\ref{tab:hyperparameters}. We pad each sample to maximum $max\_text\_len$ with a $[PAD]$ token. Similarly for each token, we pad to maintain a maximum word length $max\_word\_len$. For each experiment,
% % % we use total $\#layers$ of Transformers blocks stacked for our {\name} architecture. Further, we use the $hidden\_size$ as the number of hidden units in all the embedding and FFN layers. 
% % we use a $Dropout$ rate of $0.1$ in both transformer block and the task specific layers. Categorical cross entropy is used as the loss function with Adam ($\eta = 0.001$, $\beta_{1} = 0.9, \beta_{2} = 0.999$) optimizer \cite{kingma2014adam} in all experiments. We train our models for maximum $200$ epochs with an early-stopping criteria ($patience = 50$) based on the validation F1-score (for sentiment, POS and NER classification tasks). For machine translation, we use validation loss as the early-stopping criteria. We additionally use a learning rate scheduler to reduce learning rate to $70\%$ at plateaus with a patience of $20$ epochs. All models are trained with \textit{batch-size}$=32$.\\
% % %Models are check pointed at each epoch where validation F1 (validation loss for MT) increases (decreases) from the previous best. \\
% % \textbf{Transfer learning details.} As discussed in the section 4 of our paper, we follow two methodologies for conducting transfer learning. In fine-tuning we transfer the char-level {\name} from the pre-trained model and train the fine-tuning model with a lower learning rate of $0.0002$. In the without fine-tuning setup we freeze the pre-trained char-level {\name} model weights and learn the weights of the rests of the network with a learning rate of $0.001$.
% % \\
% % We conduct all our experiments on 1 Tesla T4 GPU.
% % % \\
% % % $\bullet$ \textbf{Named Entity Recognition:} We use Hindi and Spanish NER datasets that follow IOB nomenclature. Hindi dataset contains total 7 classes - \textit{O, B-PERSON, I-PERSON, B-PLACE, I-PLACE, B-ORGANISATION} and \textit{I-ORGANISATION}. On the other hand, Spanish NER dataset contains total 19 distinct classes.

% % % Similar to sentiment classification task, for Spanish-English POS and NER we use the dev dataset for both validation and testing. For all other datasets (Hi-En sentiment, Hi-En POS, Be-En POS, Te-En POS, Hi-En NER) we use $10-$fold cross validation where $80\%$ of the entire dataset is kept for training, $10\%$ for validation and rests $10\%$ for testing at each fold.
% % %\input{tab:dataset_stats}

% % \fi

% \section{Confusion Matrices and Error Analysis}
% We report the confusion matrices to show the label-wise performance for the sentiment classification, PoS tagging and NER in Tables \ref{fig:senticonfusion}, \ref{fig:posconfusion}, and \ref{fig:nerconfusion}, respectively. 

% % \input{supplementary:confusion}
% \begin{figure*}[ht!]
%     \centering
%     \subfloat[Hindi]{\includegraphics[scale=.17]{images/hindi_POS.pdf}} 
%     \subfloat[Spanish]{\includegraphics[scale=.17]{images/spanish_pos.pdf}}
%     \caption{Confusion matrices of {\tt HIT} on POS tasks. Due to high cardinality of output classes, we do not report for Bengali and Telugu.}
%     \label{fig:posconfusion}
% \end{figure*}

% \begin{figure*}[ht!]
%      \centering
%      \subfloat[Tamil]{\includegraphics[scale=.17]{images/tamil_sentiment.pdf}}
% 	 \subfloat[Malayalam]{\includegraphics[scale=.17]{images/malay_sentiment.pdf}}
% 	 \subfloat[Spanish]{\includegraphics[scale=.17]{images/spanish_sentiment.pdf}}
%      \caption{Confusion matrices of {\tt HIT} on sentiment tasks.}
%      \label{fig:senticonfusion}
% \end{figure*}

% \begin{figure*}[ht!]
%     \centering
%      \subfloat[Hindi]{\includegraphics[scale=.1724]{images/hindi_NER.pdf}} \hspace{2em}
%     \subfloat[Spanish]{\includegraphics[scale=.1724]{images/spanish_ner.pdf}}
%     \caption{Confusion matrices of {\tt HIT} on NER.}
%     \label{fig:nerconfusion}
% \end{figure*}

% % In this section, we study the performance of our model in greater detail by interpreting the results. We report the confusion matrices to show the performance for different majority and minority classes. Fig~\ref{fig:senticonfusion} shows that {\name} performs extremely well on the majority class \textit{Positive} and \textit{Negative}. Another interesting observation (Fig~\ref{fig:senticonfusion}) is that {\name} can detect the distinguished linguistic characteristics for Dravidian languages (Tamil and Malayalam). For these two datasets, {\name} classifies the \textit{non-Tamil} and \textit{non-Malayalam} classes with $69\%$ and $81\%$ accuracy respectively, much more than the other baselines. We perform a detailed qualitative analysis in Table~\ref{tab:error} on few instances to understand our model's behavior at granular level. We take the example of Hindi text \textit{``safal videsh yatra ke liye badhai ho sir"}, which translates to \textit{``Congratulations for the successful foreign trip sir"} in English. This text wishes good luck to a person, which can be thought as a positive sign. It is not hard to understand that the most positive vibe is attributed by the phrase \textit{``badhai ho sir"}, which translates to \textit{``congratulations sir"}. To validate our hypothesis, we use a gradient based interpretation technique. We use Grad-CAM as proposed by \cite{Selvaraju_2019}, which makes use of gradients of neural networks to show each neuron's importance to the final output. Due to hierarchical and modular nature of {\name}, we are able to extract the intermediate word level representations learnt by the character level sub-network and compute the gradient of loss of the actual class w.r.t these representations. The magnitude of gradient shows the impact of each word on the final output. Fig ~\ref{fig:interpretsentiment1}(a) validates our hypothesis. Further, the attention plot of Fig ~\ref{fig:interpretsentiment1}(c) shows high attention weights of all the words with `badhai' which strengthens our hypothesis. To further showcase the robustness of our model, we perturb the original text to \textit{``safal videsh yatra ke liye badhaaii ho sir!!"} and run the same procedure. {\name} predicts positive class for the perturbed text as well. It is interesting to notice from Fig~\ref{fig:interpretsentiment1}(b,d) that the word importance quickly shifts towards `!!' which emphasize the sentiment polarity of the text. Further, character level attention plot in ~\ref{fig:interpretsentiment1}(e,f) shows the phonetic similarity of the words \textit{`badhai'} and \textit{`badhaaii'}, although the word \textit{`badhaaii'} was not part of our actual vocabulary. \\



% % \begin{figure}[htb]
% %      \centering
% %      \subfloat[]{\includegraphics[scale=.5]{images/grad_plot_negative.png}} \\\
% % 	 \subfloat[]{\includegraphics[scale=.25]{images/original_word_attention_negative.pdf}}
% %      \caption{Interpretation of a negative Hi-En sentiment prediction (a) Grad-CAM;\,(b) Word attention plot. The high gradient and attention weight values of word \textit{`media'} shows its impact on the overall prediction.}
% %      \label{fig:interpretsentiment2}
% % 		%\vspace*{-0.5cm}
% % \end{figure}

% % We take the example 3 from Table~\ref{tab:error}(a) as a negative example, where the {\name}  predicts a neutral text as negative. Upon interpreting the behavior of our model (Fig~\ref{fig:interpretsentiment2}), we understand that our model understand the subtle rudeness in the text through the phrase \textit{`karo'}, which means \textit{`do it'}. Also, the word \textit{`media'} is used here in the bad light, which our model is able to extract.


% % \if 0
% % \begin{figure*}
% %      \centering
% %      \begin{minipage}
% %      \centering
% %          \includegraphics[scale=.15]{images/hindi_sentiment.pdf}
% %          \subcaption{Hi-En Sentiment}
% %          %\label{fig:hisenti}
% %      \end{minipage}
% %      %\hfill
% %      \begin{minipage}
% %      \centering
% %          \includegraphics[scale=.15]{images/tamil_sentiment.pdf}
% %          \subcaption{$y=3sinx$}
% %          %\label{fig:three sin x}
% %      \end{minipage}
% %      %\hfill
% %      %\newline
% %      \begin{minipage}
% %      \centering
% %          \includegraphics[scale=.15]{images/malay_sentiment.pdf}
% %          \subcaption{$y=5/x$}
% %          %\label{fig:five over x}
% %      \end{minipage}
% %         \caption{Three simple graphs}
% %         \label{fig:three graphs}
% % \end{figure*}
% % \fi




% % \if 0
% % We can observe that {\em I1} and {\em I2} are cases where {\name} predicted the correct output while CS-ELMo did not. To dive deeper, we can observe that according to Grad-CAM, the words {\em modi} and {\em preiminister} (phonetic equivalent of {\em Prime Minister}) are being paid more attention to and {\name} is able to connect the word {\em jigood} (equivalent to {\em good}) to the Prime Minister and pushing the polarity towards Positive. Further, in the case of {\em I4} we can see that {\name} appears to have gotten it wrong. However, upon further inspection it can be noted that the words {\em kya baat} are being emphasised here and they should be since this is a common expression in Hindi signifying {\em Way to go!}, which expresses positive sentiment and {\name} is able to capture it. In a similar manner, in {\em I3}, the phrase {\em bhai salman bhai} is a common positive term of endearment in Hindi, which {\name} is able to identify, but CS-ELMo is not. {\name} has an advantage over CS-ELMo while incorporating character-level interactions due to {\em FAME}, which may be the reason why it is able to capture language-specific sentiment for phonetically similar words.

% % Further we study the class-wise performance of the Hi-En (Figure: \ref{fig:Hi-EnSentConf}) and Ma-En (Figure: \ref{fig:Ma-EnSentConf}) through their Confusion matrices for {\name} and CS-ELMo. For Hi-En task, we can observe that {\name} performs much better than CS-ELMo for the largest majority class ({\em Positive}) and the minority class ({\em Negative}), however for {\em Neutral} cases our performance dips a bit, which may be attributed to {\name}'s ability to capture language specific sentiments. For Ma-En task, {\name} performs better than CS-ELMo in the top 3 majority classes, however its performance dips for {\em Positive} and {\em Mixed Feelings} cases.
% % \fi

% %On the syntactic task of PoS, {\name} performs extremely well on most classes. For Sp-En {\name} detects punctuations (\textit{PUNCT}) with $100\%$ accuracy. Similarly, in Hi-En our model detects negations (\textit{PART\_NEG}) and  the Wh-words (\textit{PRON\_WH}) with $100\%$ accuracy. On the other hand, on NER task, the overall performance of {\name} is relatively poor as compared to other tasks. In NER we observe that our model is able to detect the beginning of an entity more accurately than the inside of an entity. However for Sp-En, transferring knowledge from higher level semantic tasks like sentiment classification helps in overcoming this issue for {\name}. \\

% We similarly perform qualitative analysis on the MT task where our model shows superior performance as compared to the baselines. In example 1 of Table~\ref{tab:error:supp} (d), {\name} translates the English text `\textit{`Licencing and import policies were liberalise''} to \textit{``Licencing aur policies liberal the |''}. Although this prediction has very low BLEU score when evaluated against the target, this example shows an interesting observation. %The Hindi phrase \textit{``udhar le leta hu"} translates to \textit{``I will borrow"}, which strongly resembles with the source text. 
% The overall translation is a contextually meaningful sentence in Hindi. Further {\name} translates the phrase \textit{`were liberalise'} to \textit{`liberal the'}. In Hindi, \textit{`the'} represents past tense. Another interesting observation is the ability of {\name} to copy texts from source to predicted text. Even without having an explicit copying mechanism~\cite{see2017get}, {\name} is able to understand the key phrases that co-occur in both Hindi and English, like, numeric and proper nouns and copies these tokens while generating. This shows how our model can also be used in conditional generation of texts. It also ends the sentence with |, which is a common punctuation widely used as a full stop in Hindi texts.
% % \input{tab:hyperparameters}

% \input{supplementary-tab-error-examples}
% \newpage

% \bibliographystyle{acl_natbib}
% \bibliography{acl2021}

% \end{document}
