# Supplementary material for: HIT: A Hierarchically Fused Deep Attention Network for Robust Code-mixed Language Representation
Source: arXiv:2105.14600 source file (2021-05-30)
Supplement: Supplementary file 2 [file supplementary-confusion.tex]

% \begin{figure}
% \centering
% \includegraphics[width=0.5\textwidth]{images/Hi-En Sentiment HIT CS-ELMo.png}
% \caption{Confusion Matrix of Sentiment Classes for Hi-En task. Left: {\name} and Right: CS-ELMo}
% \label{fig:Hi-EnSentConf}
% \end{figure}

% \begin{figure}
% \centering
% \includegraphics[width=0.5\textwidth]{images/Ma-En HIT CS-ELMo.png}
% \caption{Confusion Matrix of Sentiment Classes for Ma-En task. Left: {\name} and Right: CS-ELMo}
% \label{fig:Ma-EnSentConf}
% \end{figure}

\begin{figure*}[t]
    \centering
    \subfloat[Hindi]{\includegraphics[scale=.1724]{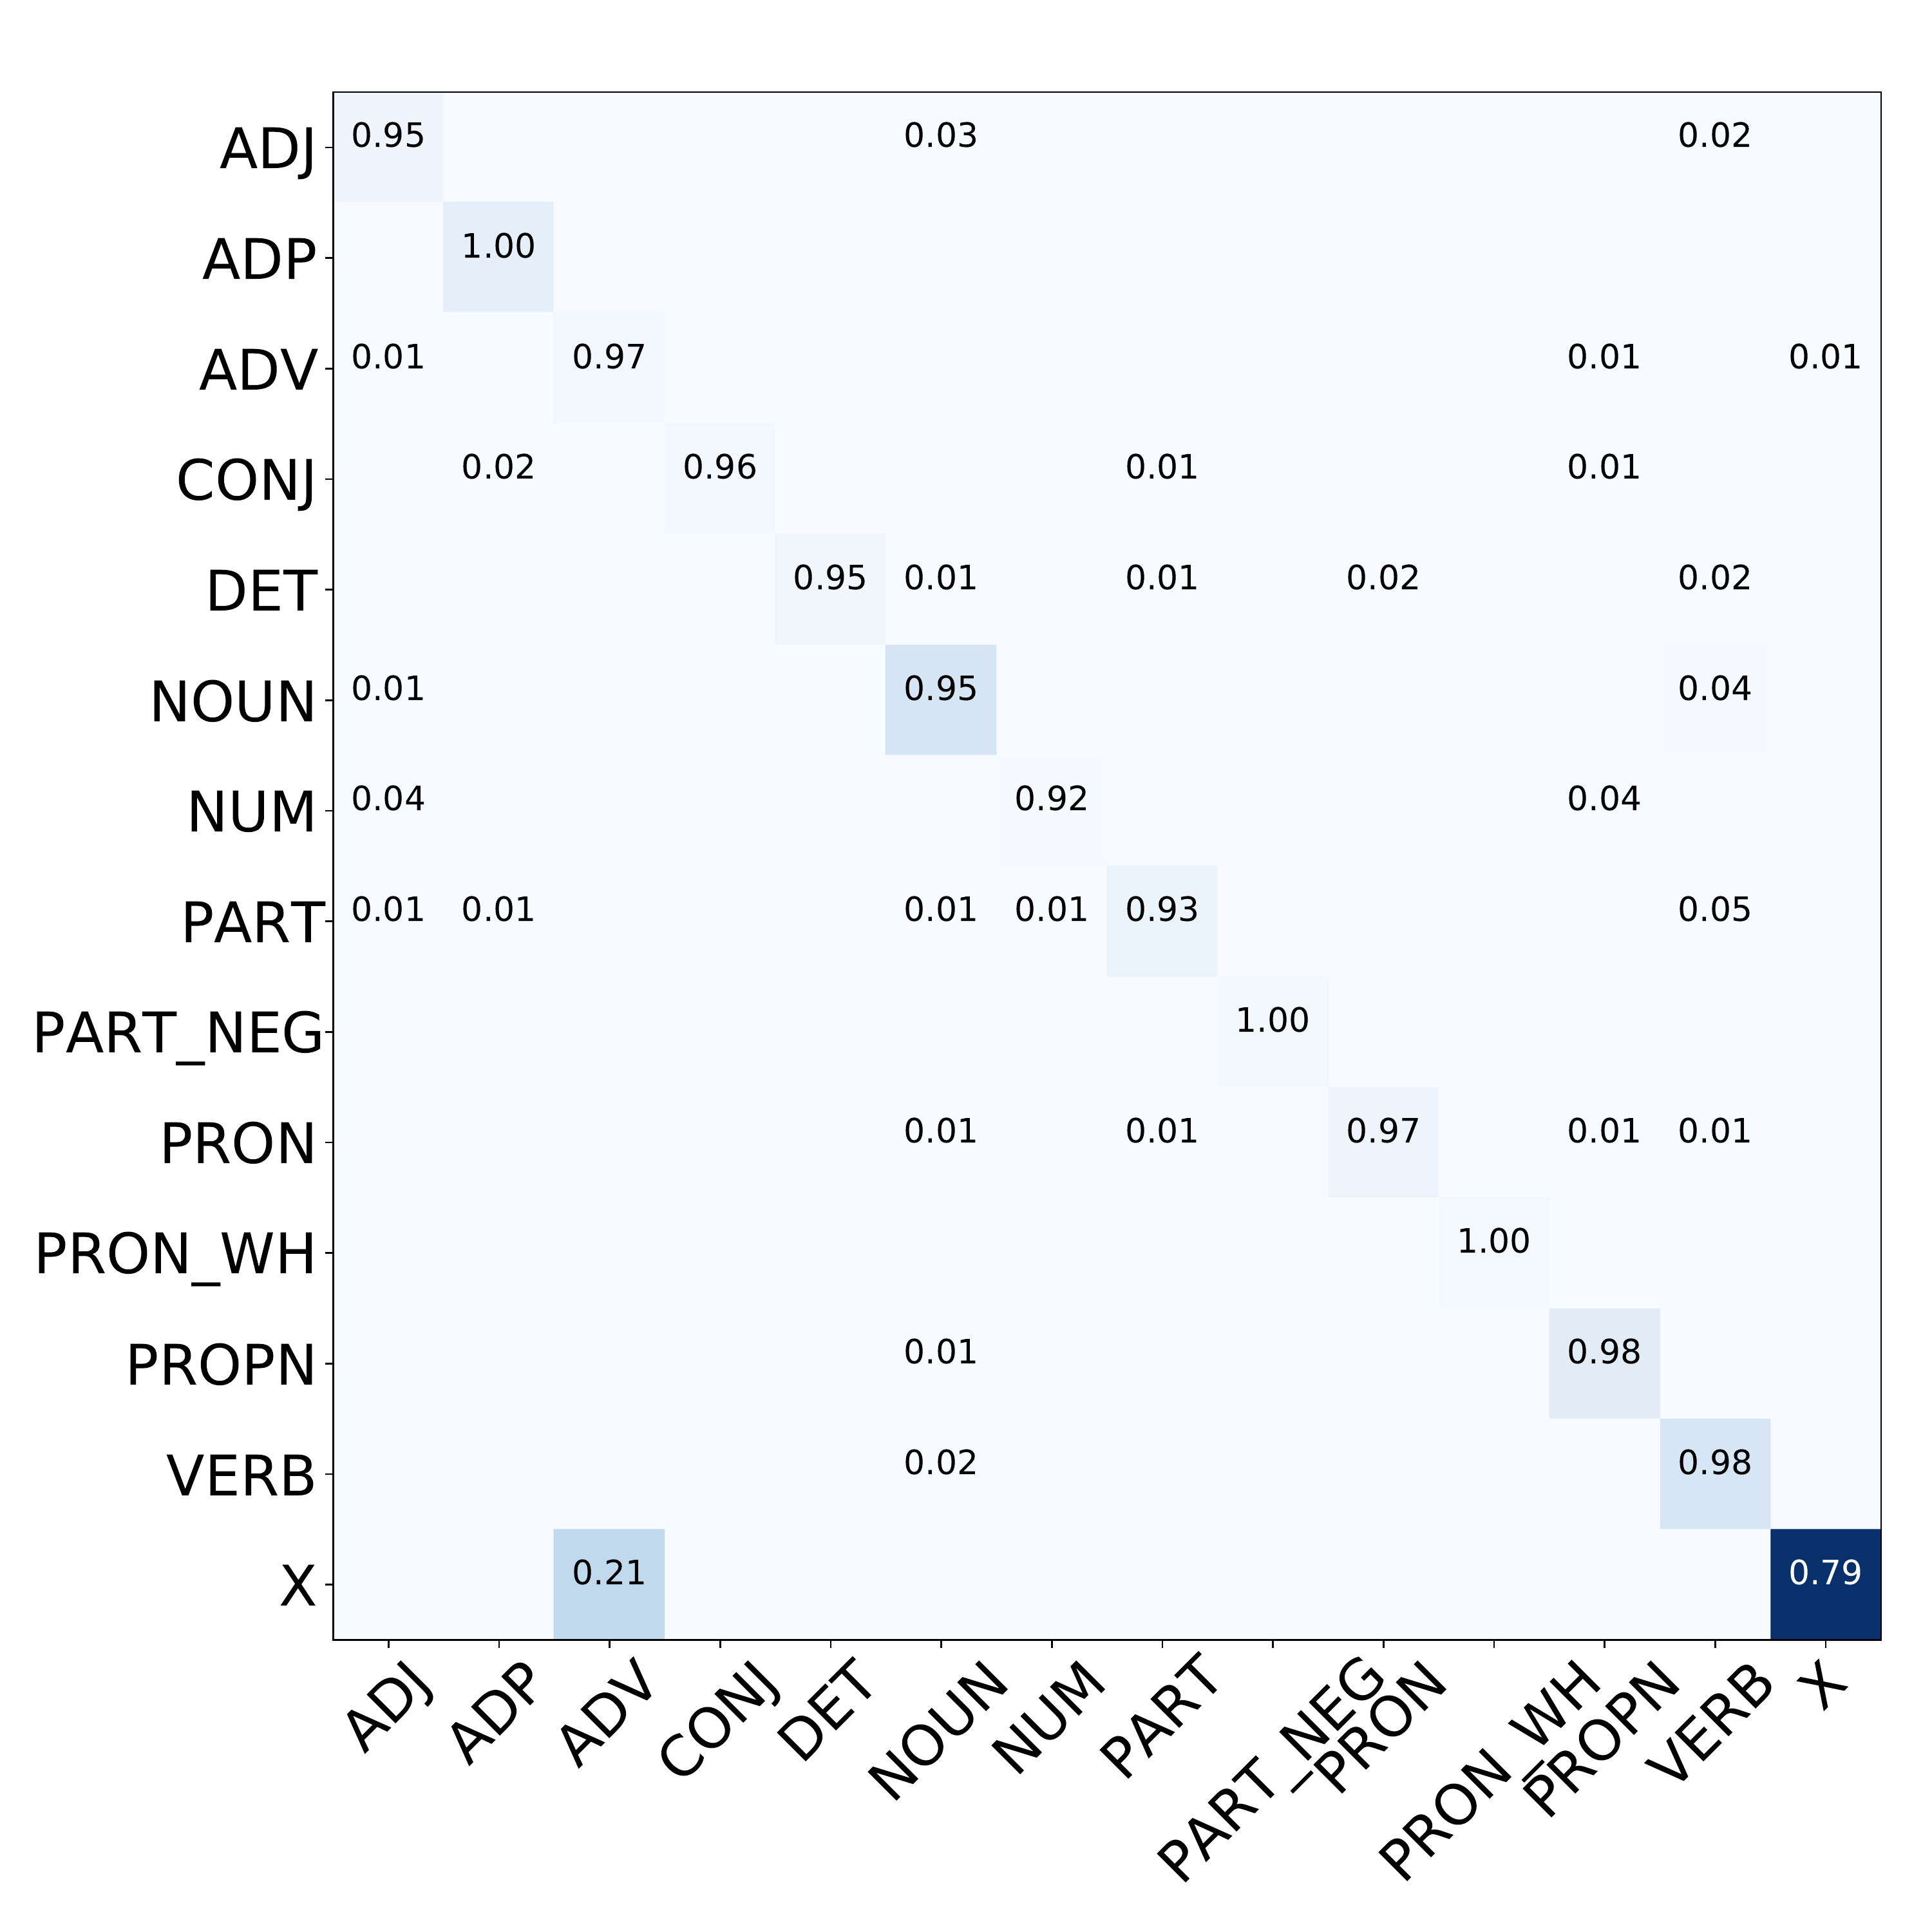}} 
    % \hspace{2em}
    
    \subfloat[Spanish]{\includegraphics[scale=.1723]{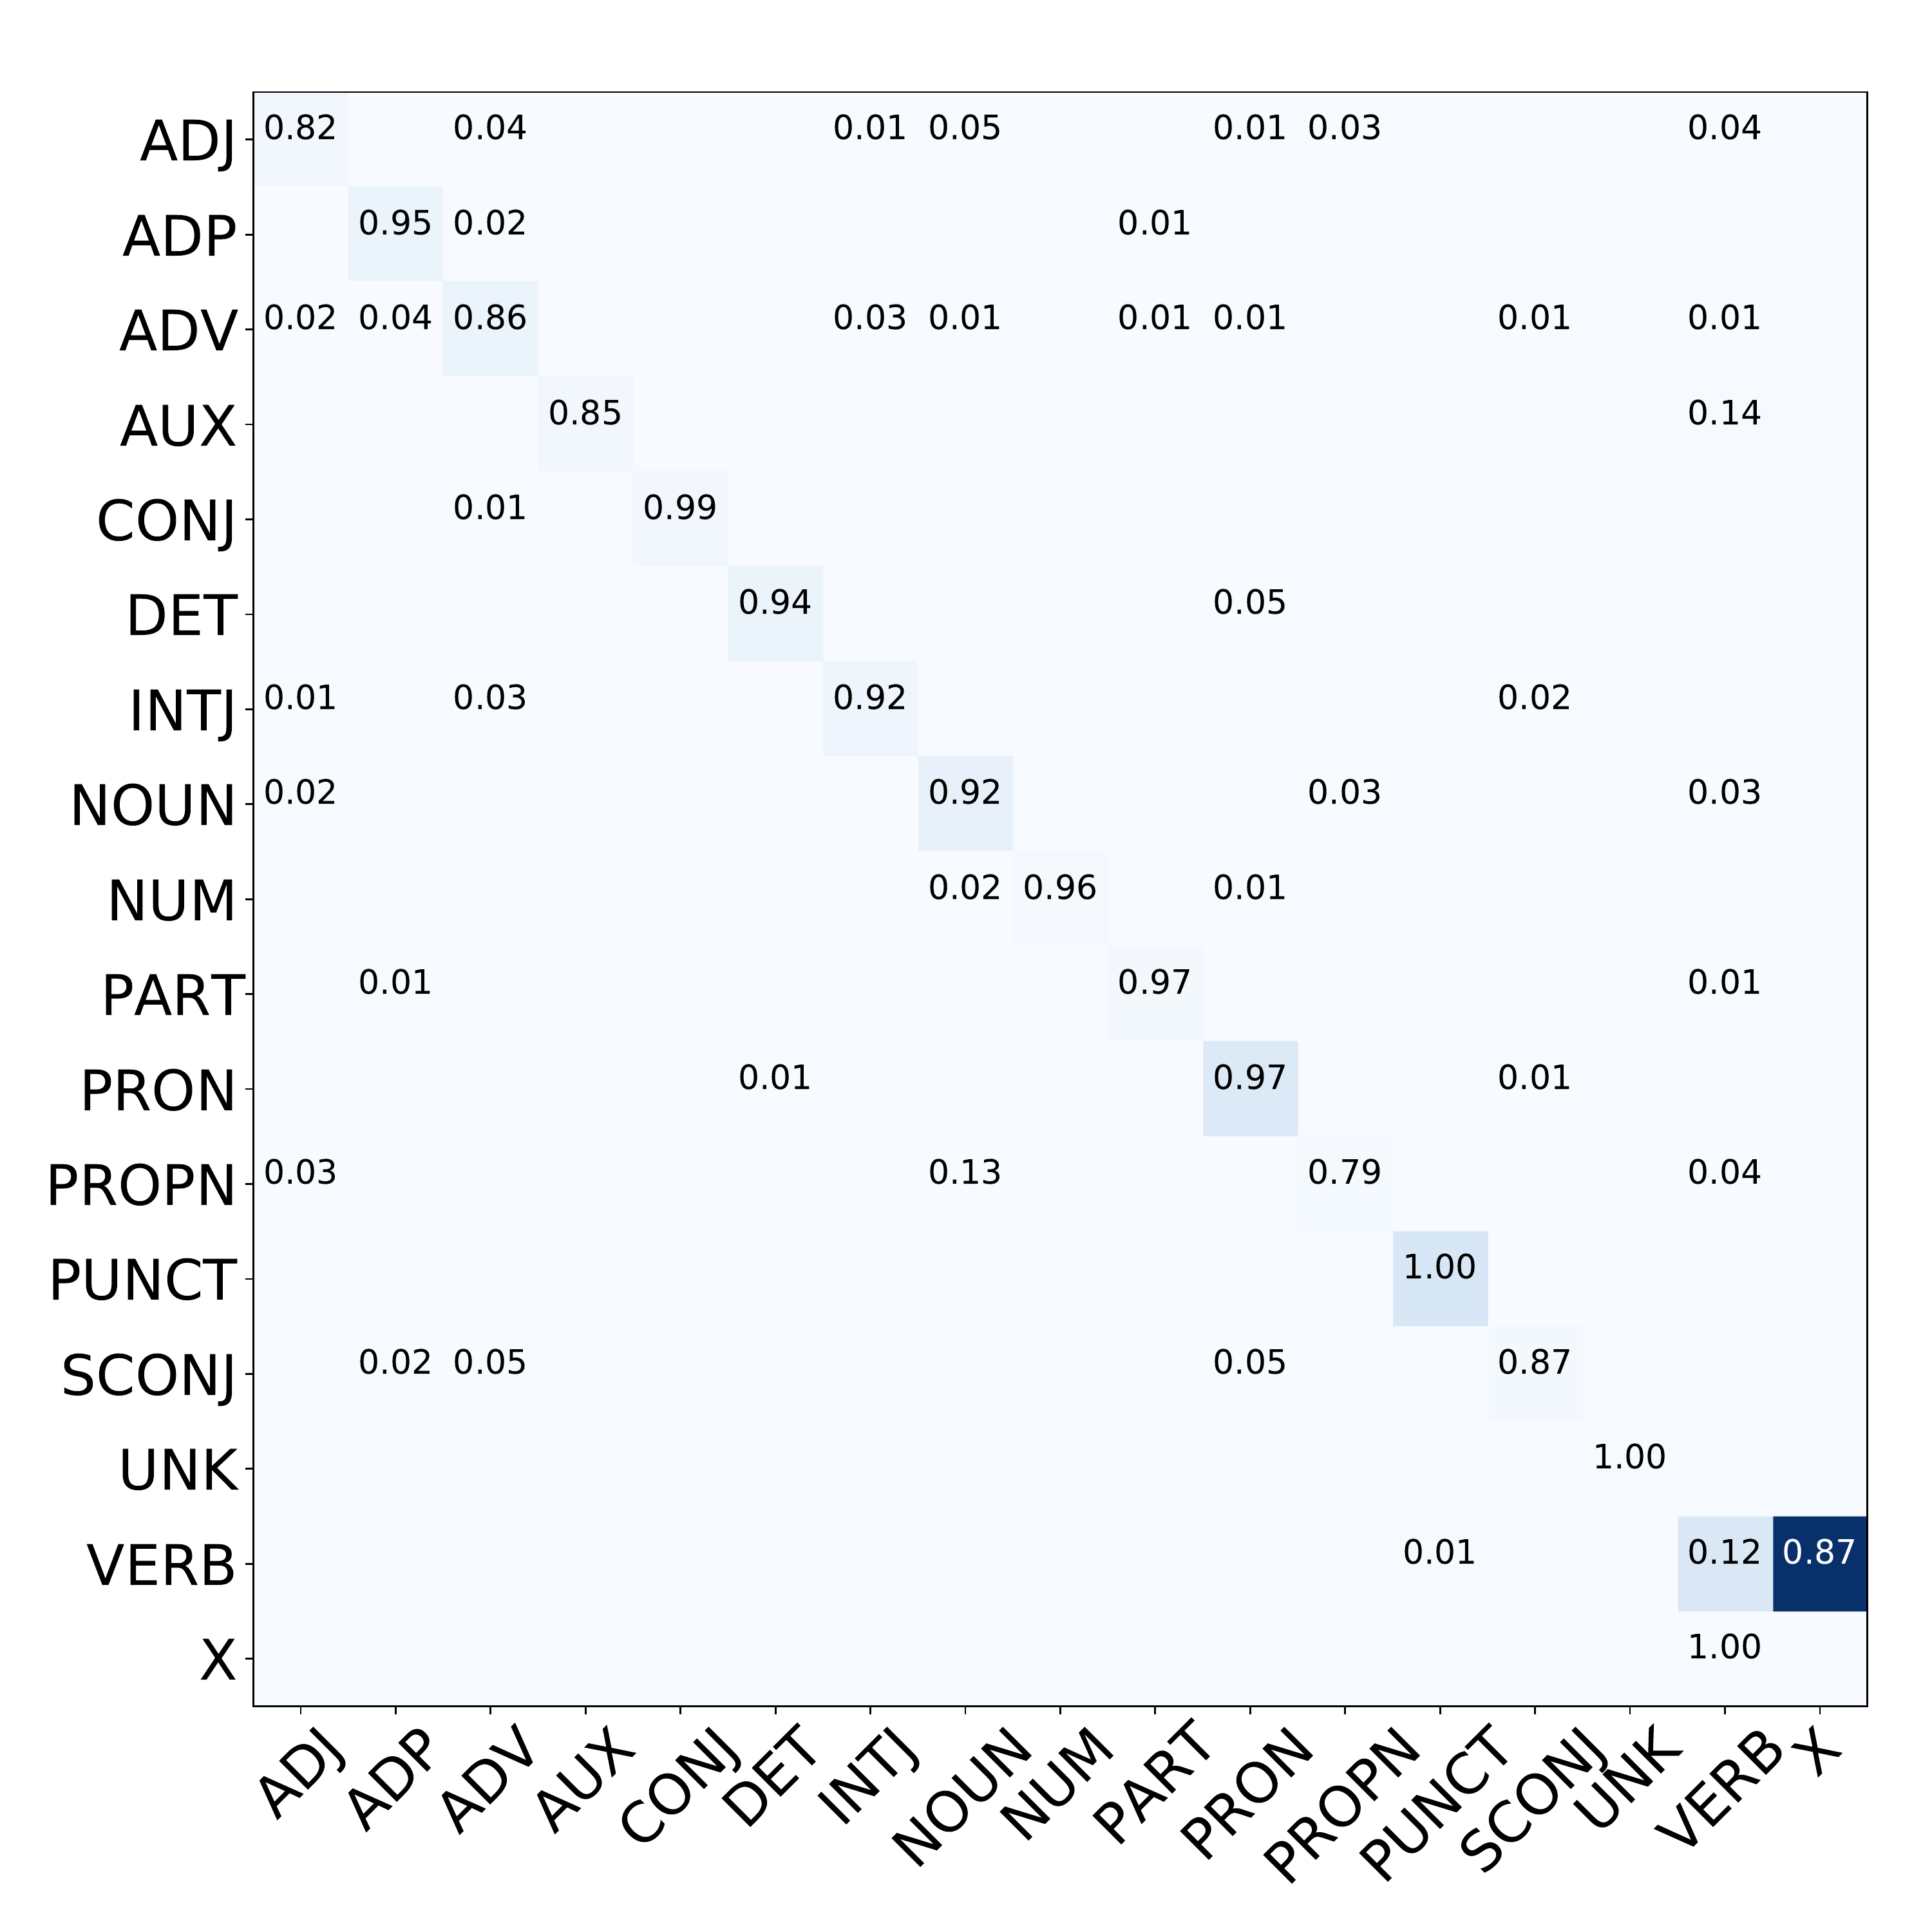}}
    \caption{Confusion matrices of {\tt HIT} on POS tasks. Due to high cardinality of output classes, we do not report for Bengali and Telugu.}
    \label{fig:posconfusion}
\end{figure*}

\begin{figure*}[ht]
     \centering
     \subfloat[Tamil]{\includegraphics[scale=.17]{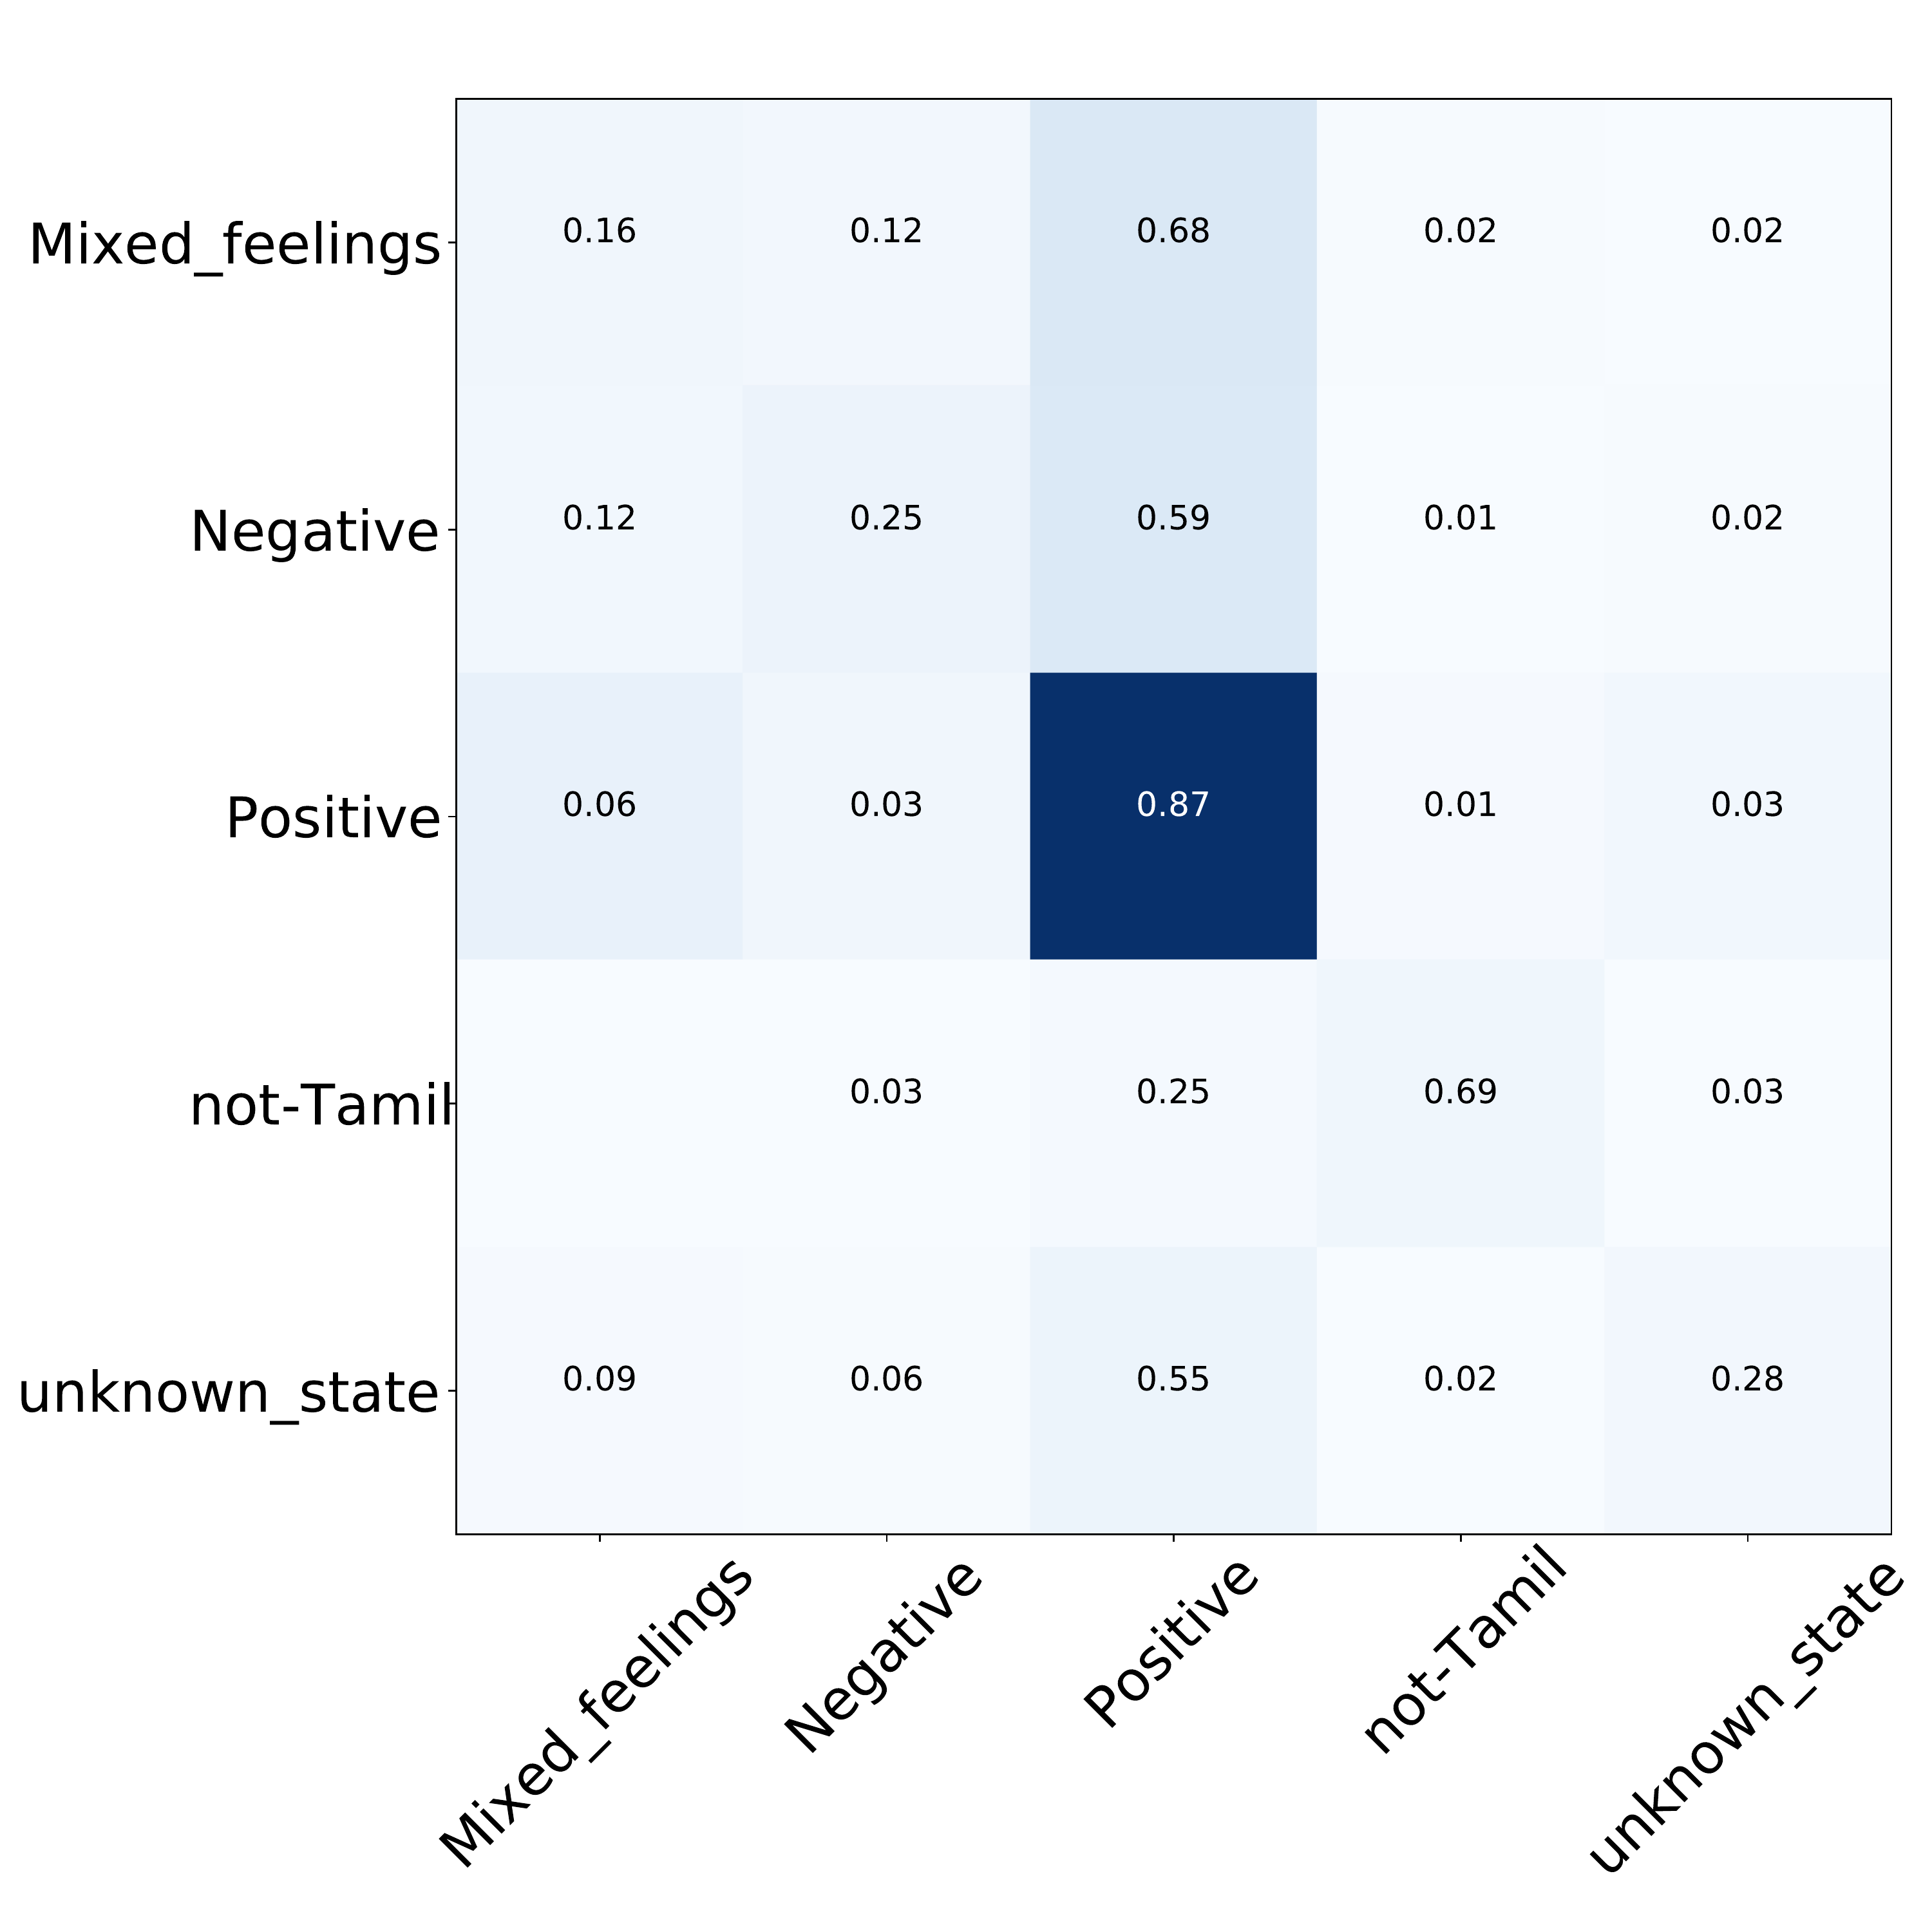}}
     
	 \subfloat[Malayalam]{\includegraphics[scale=.17]{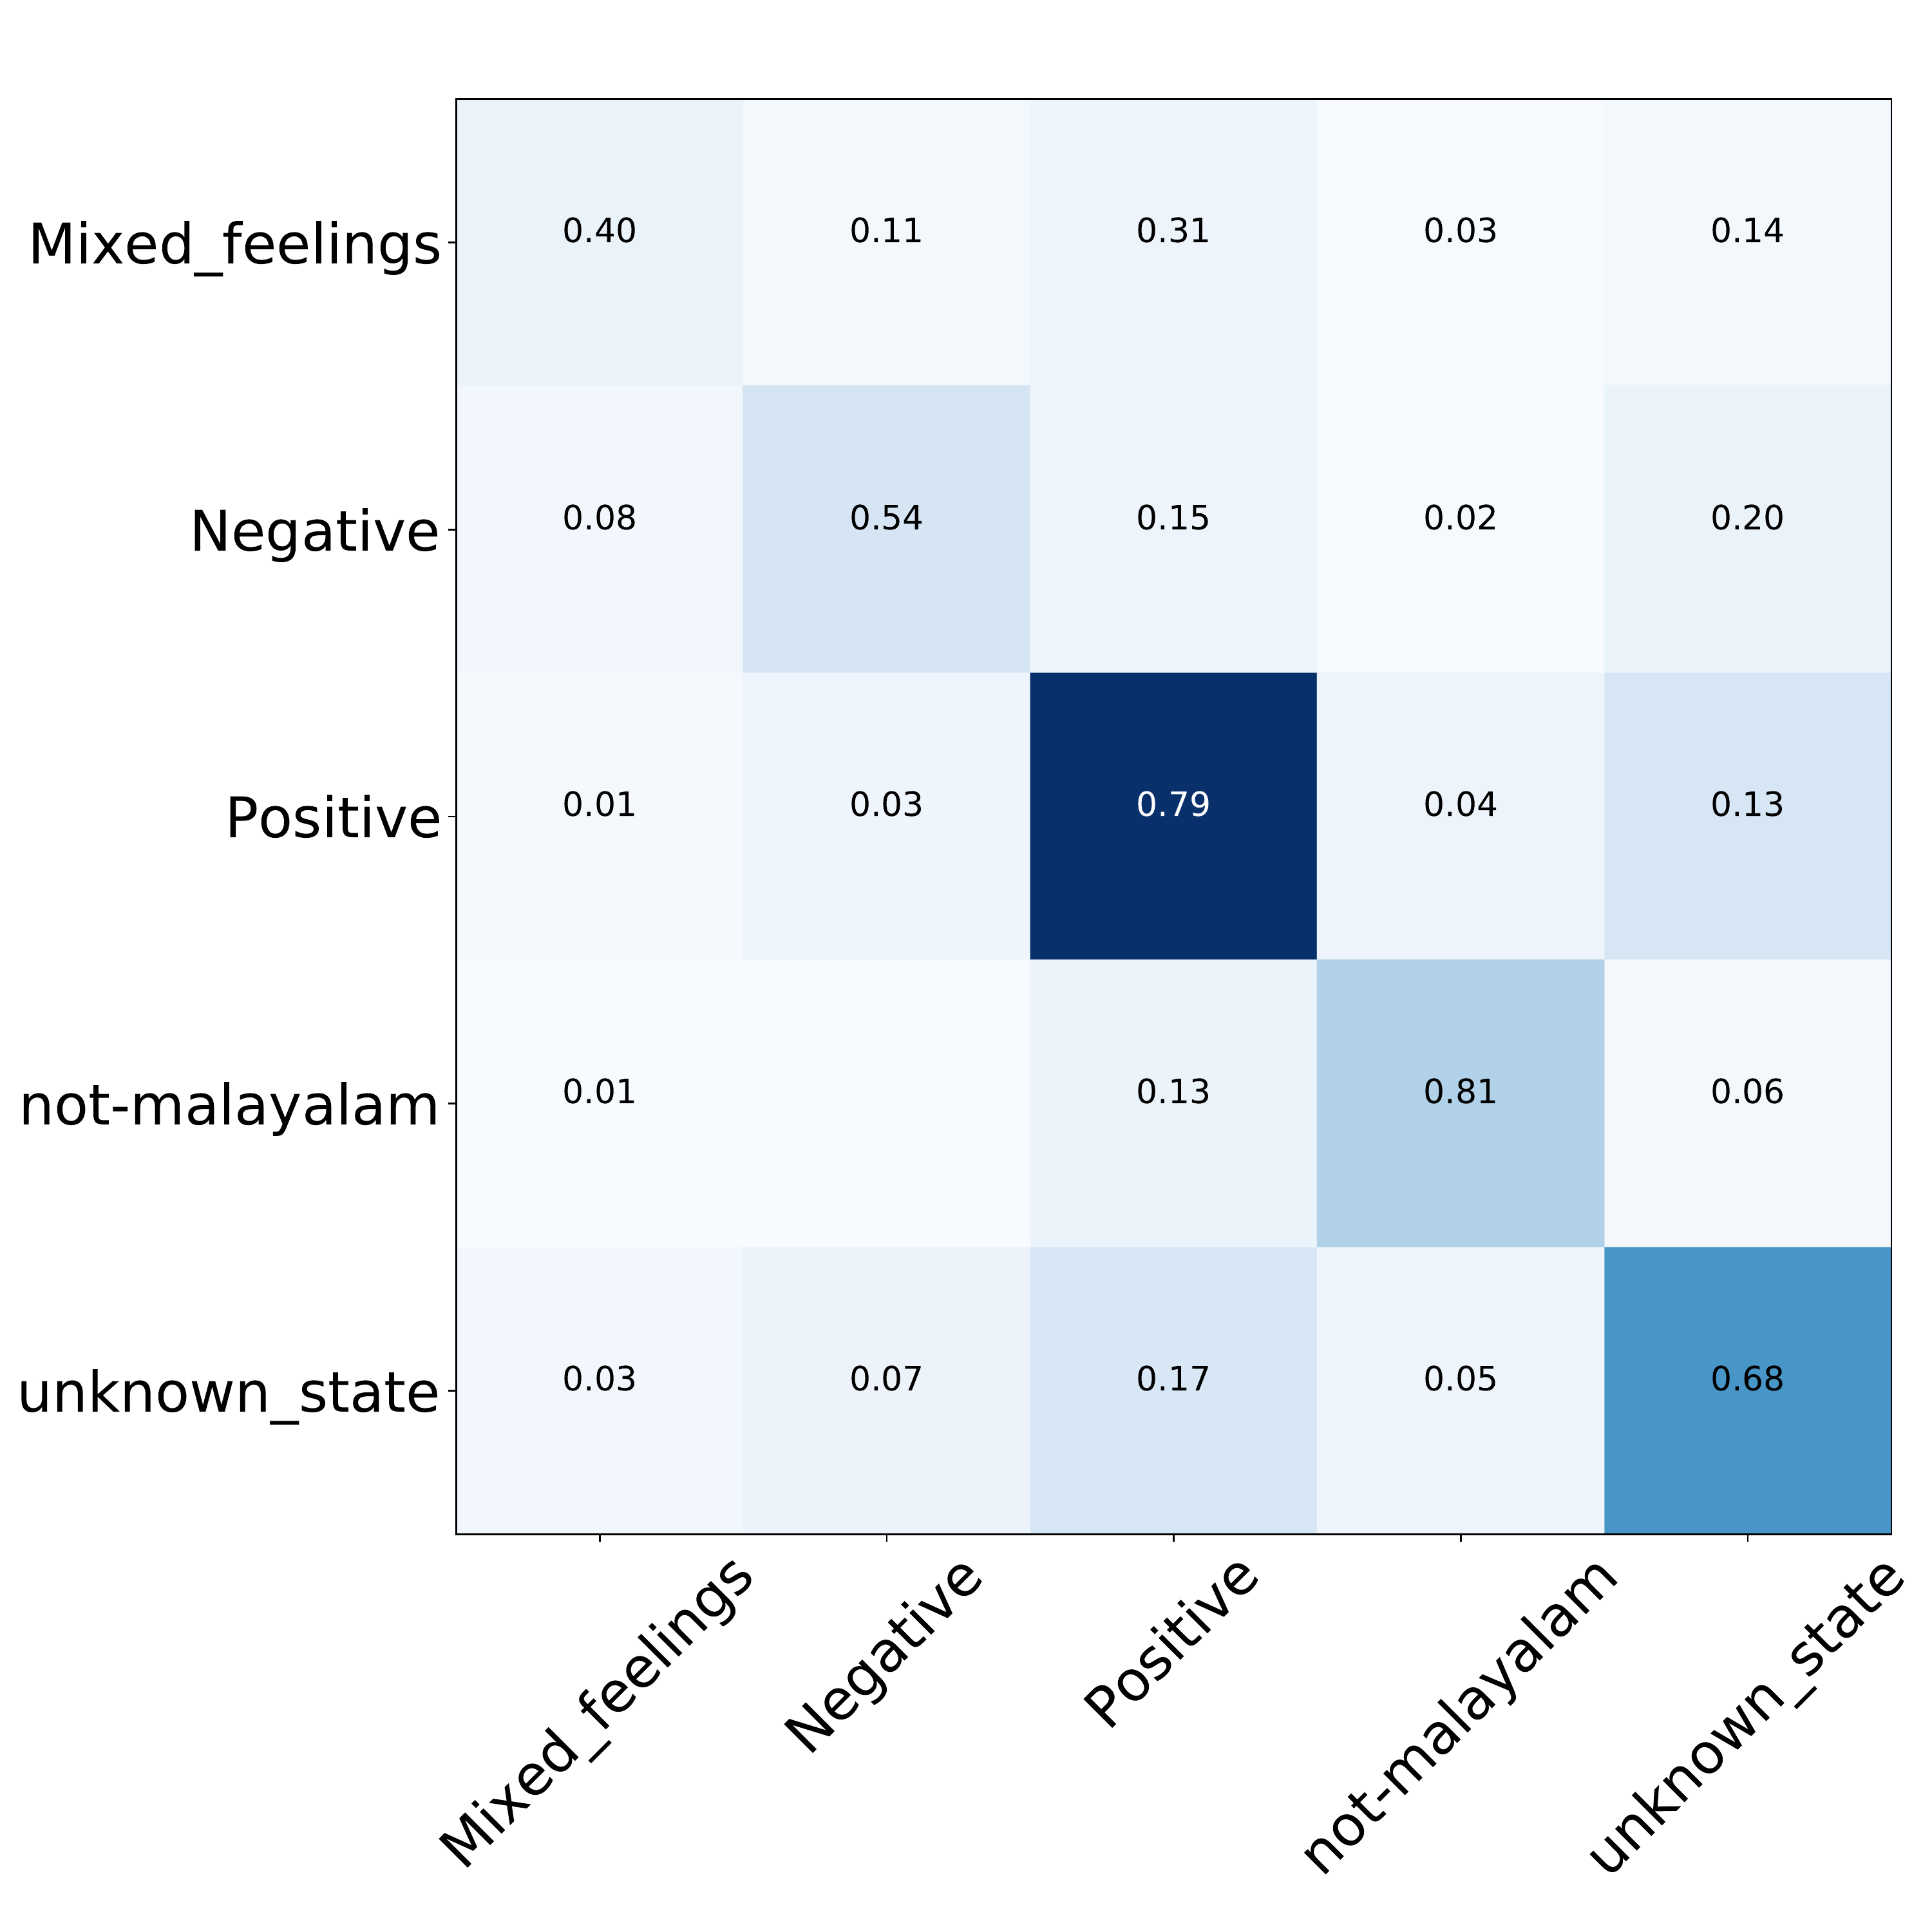}}
	 
	 \subfloat[Spanish]{\includegraphics[scale=.17]{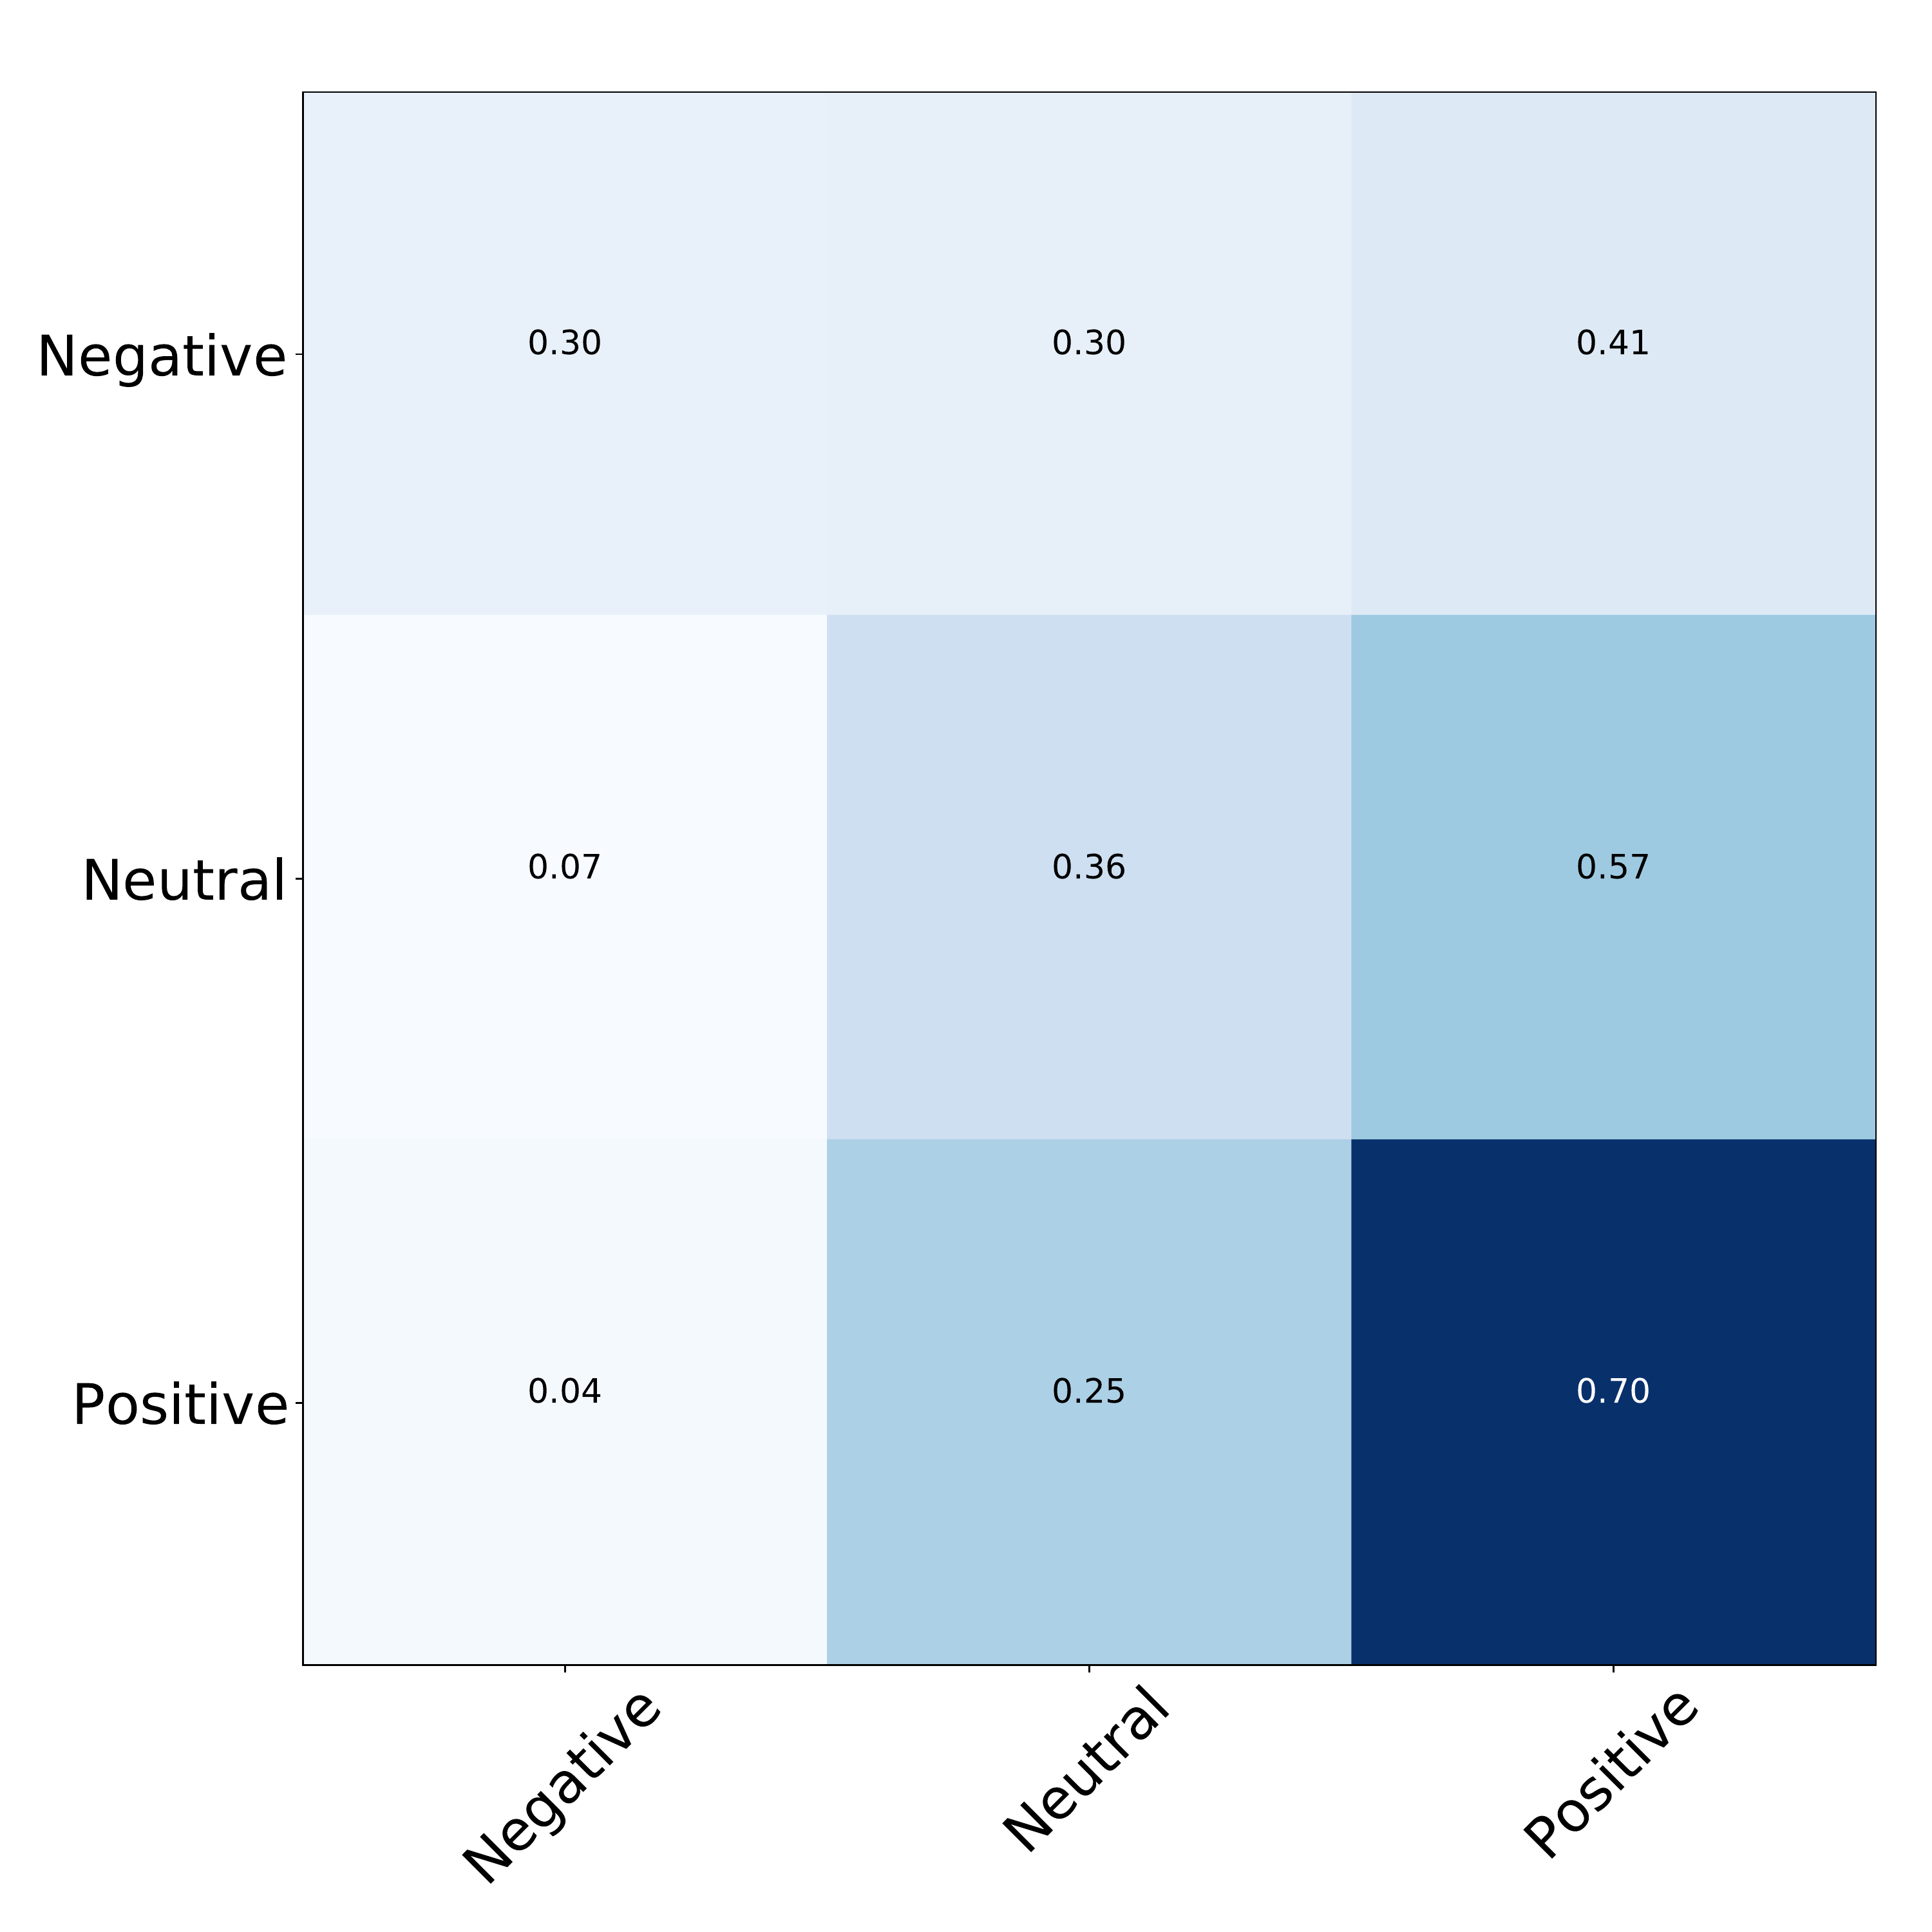}}
     \caption{Confusion matrices of {\tt HIT} on sentiment tasks.}
     \label{fig:senticonfusion}
\end{figure*}

\begin{figure*}[t]
    \centering
     \subfloat[Hindi]{\includegraphics[scale=.1724]{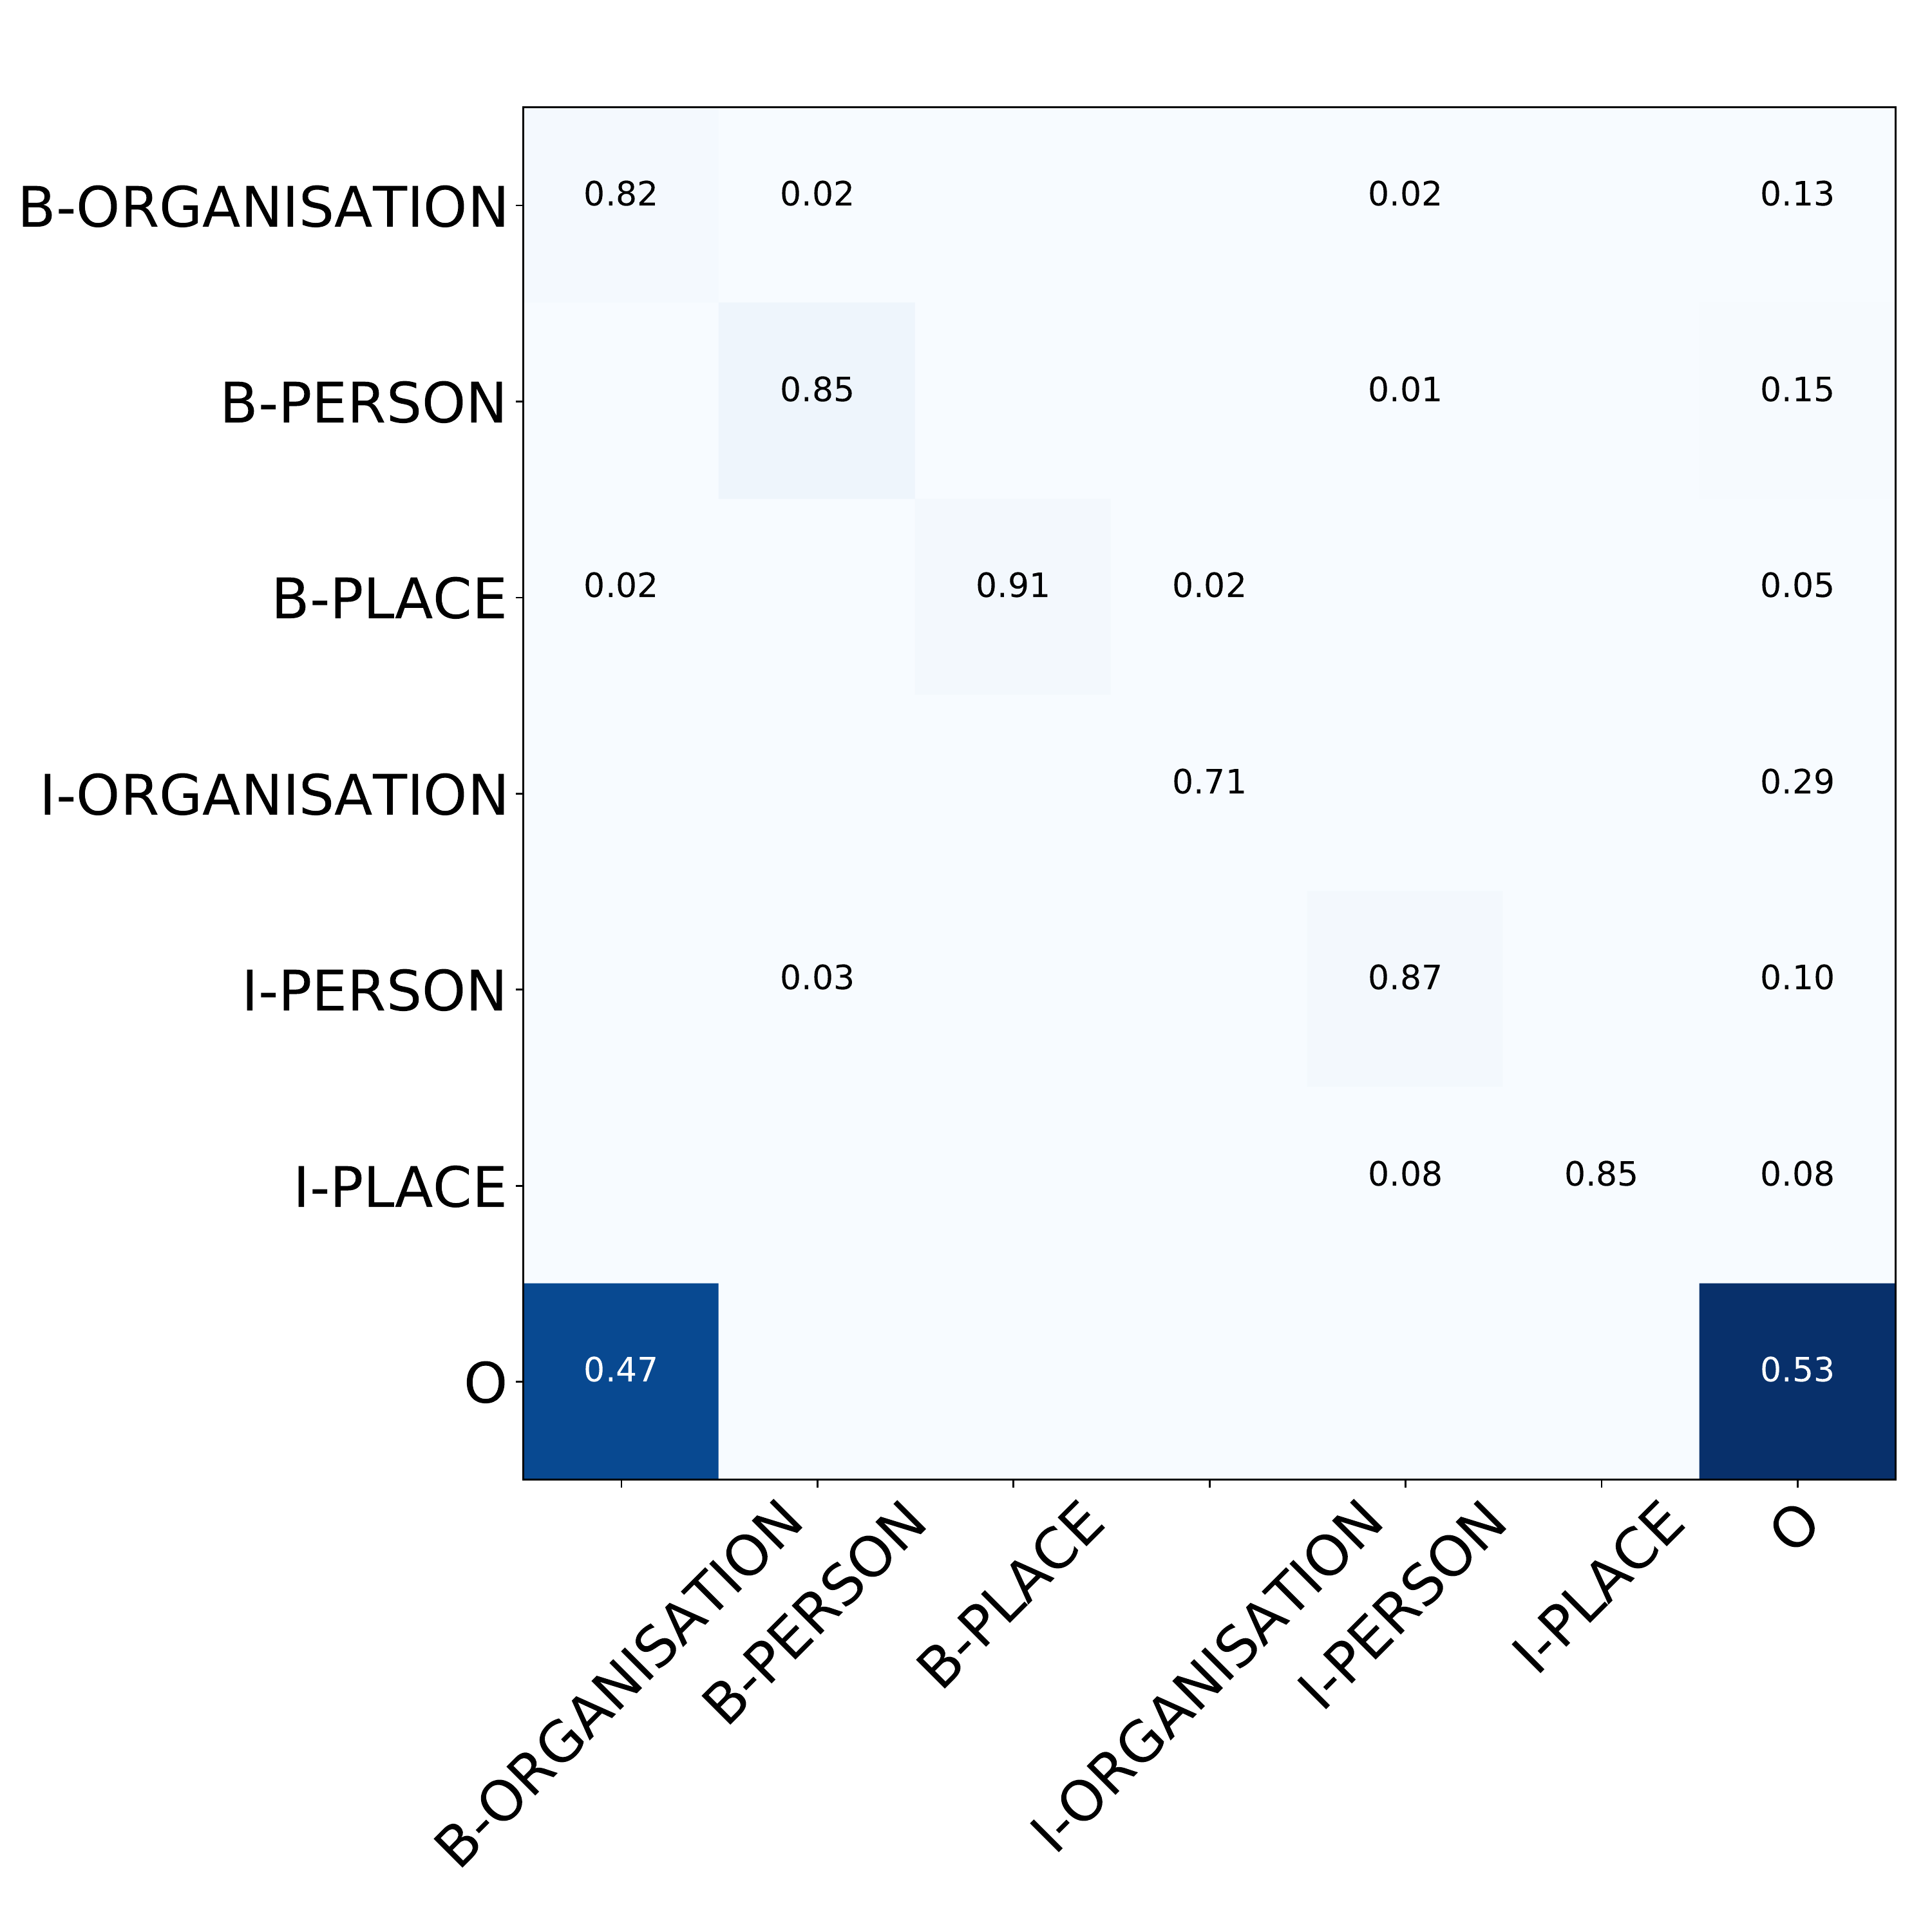}} \hspace{2em}
    \subfloat[Spanish]{\includegraphics[scale=.1724]{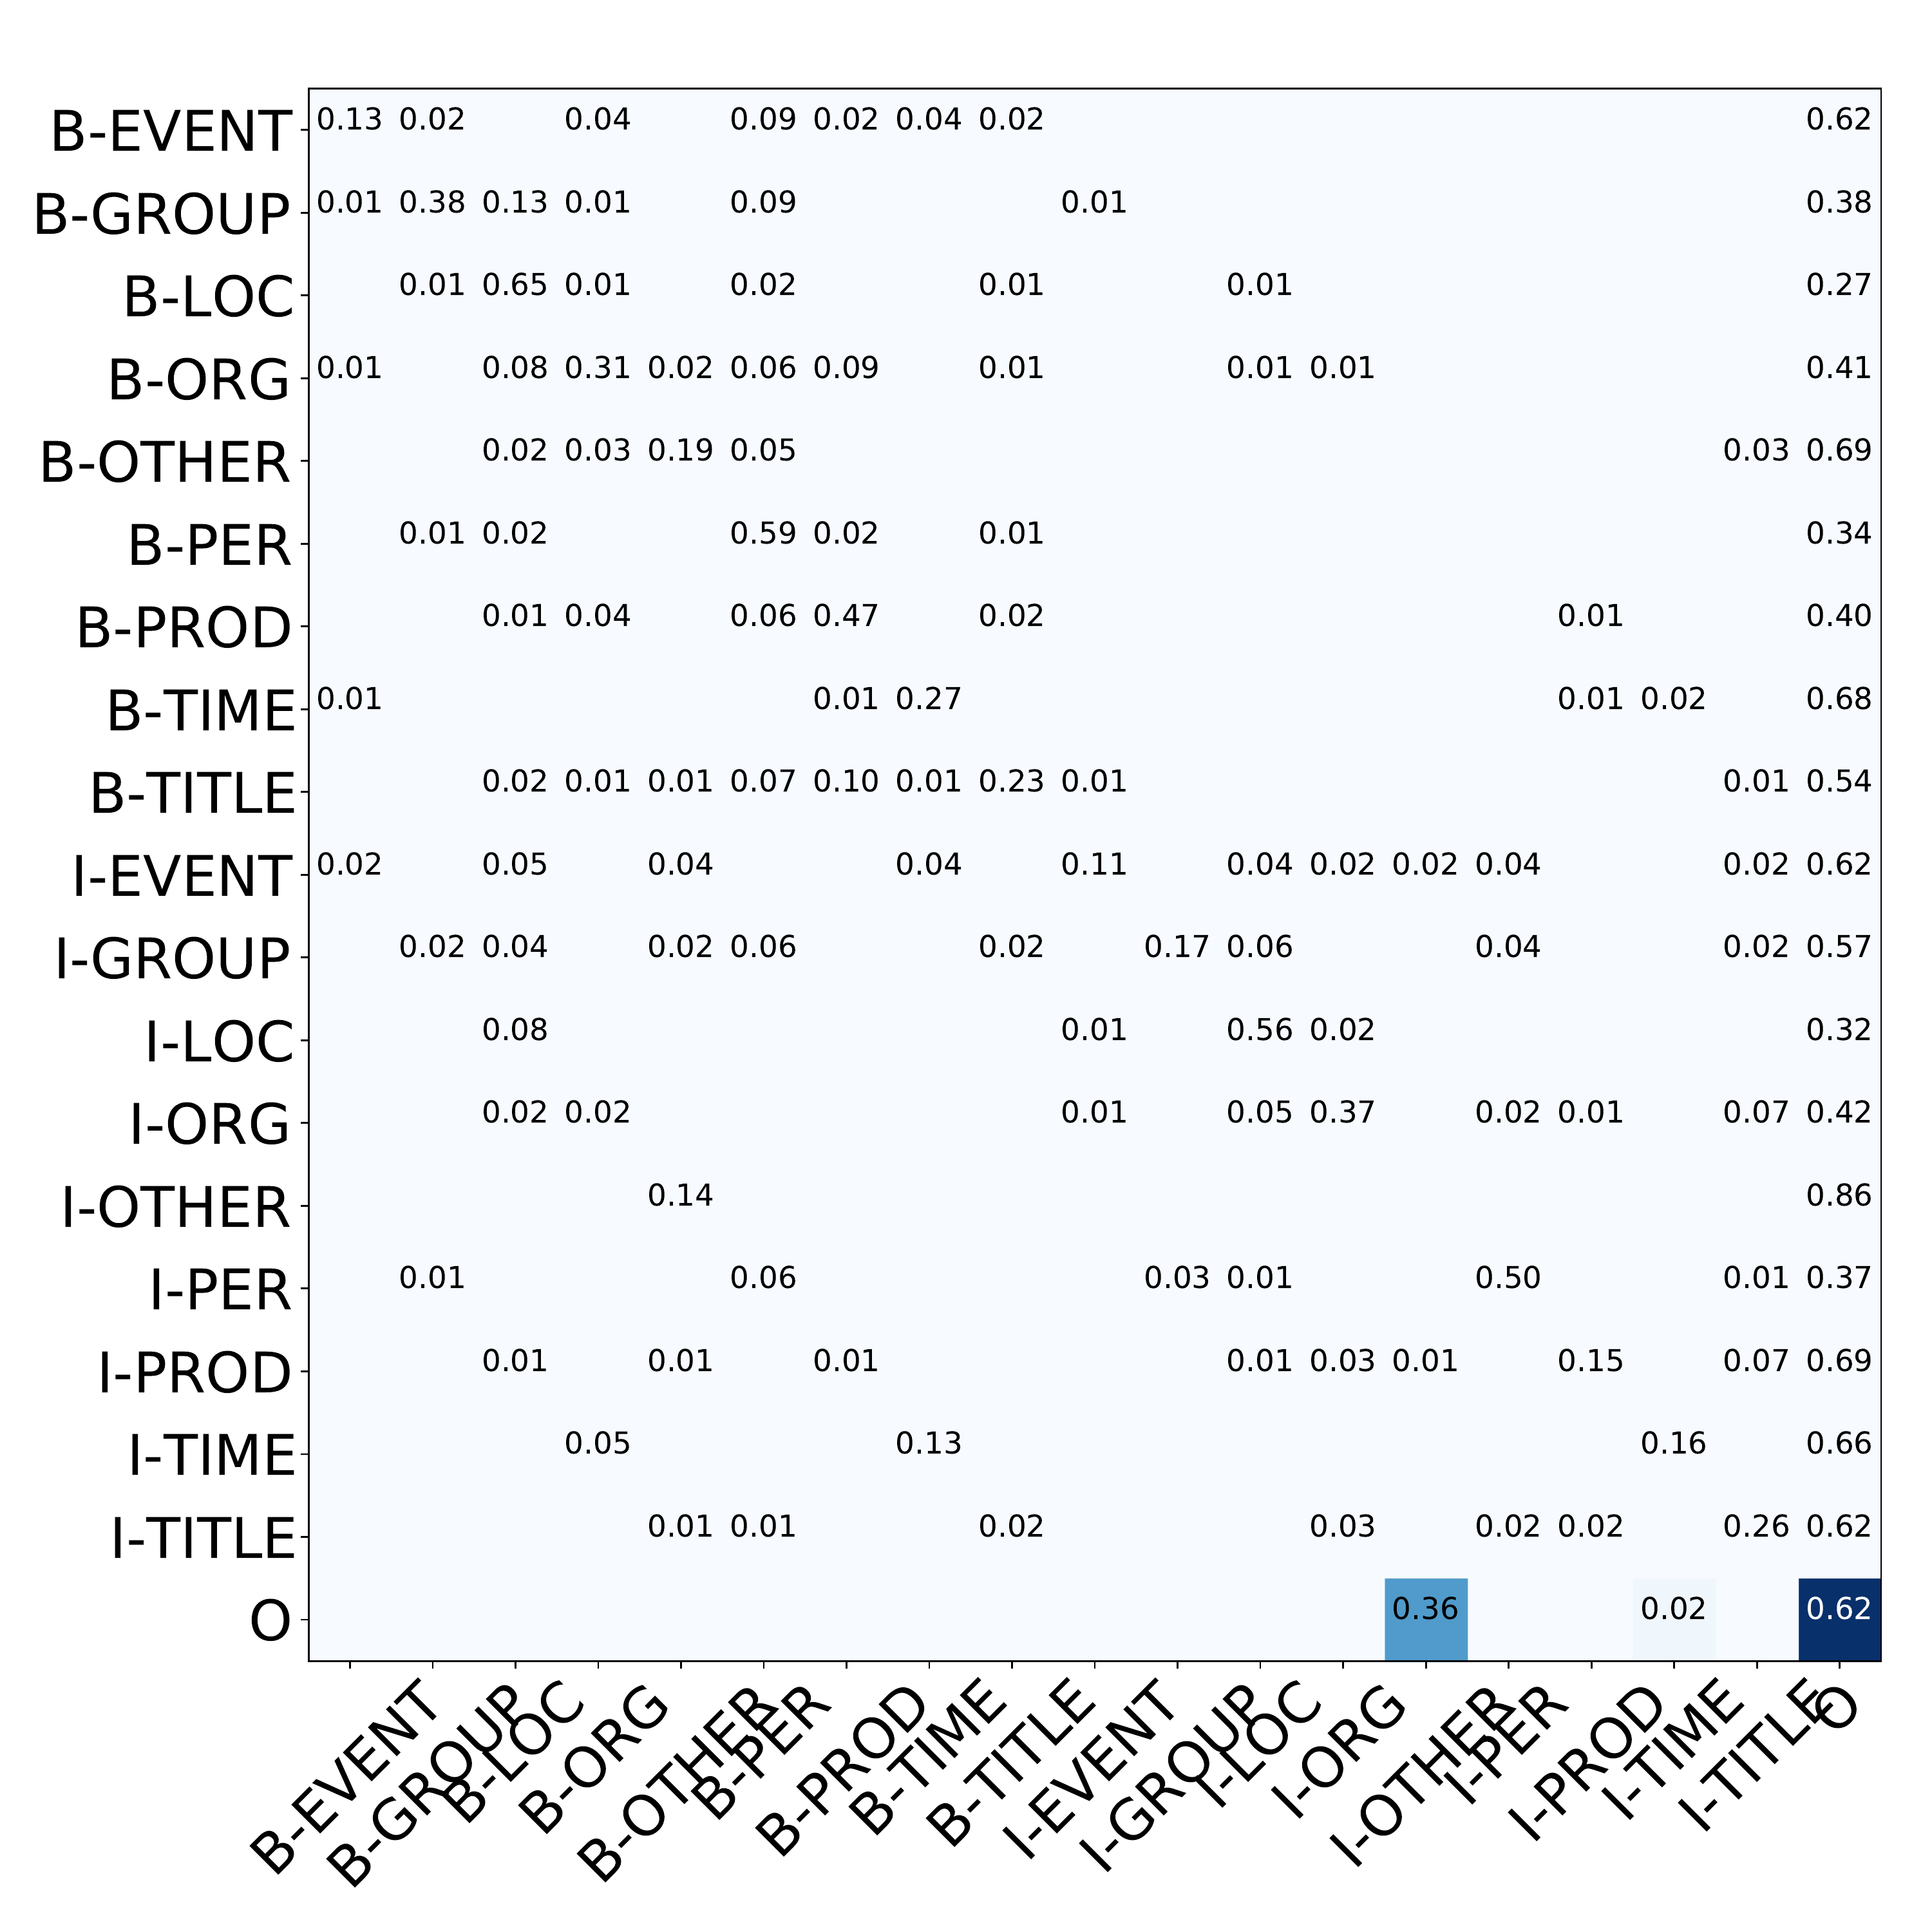}}
    \caption{Confusion matrices of {\tt HIT} on NER.}
    \label{fig:nerconfusion}
\end{figure*}
